# Supplementary material for: Reciprocal Normalization for Domain Adaptation
Source: arXiv:2112.10474 source file (2021-12-20)
Supplement: Supplementary file 1 [file Method.tex]

\section{More details about RN}
%%%
\subsection{Motivation}
We re-state the motivation of the proposed Reciprocal Normalization (RN) in a clearer way.
In the context of Unsupervised Domain Adaptation (UDA), there are two drawbacks of Batch Normalization (BN): 1) sharing the same mean and variance in different domains is unreasonable and can result in distortion of distribution and domain-specific knowledge; 
2) BN neglects domain discrepancy and cannot conduct domain alignment explicitly, which can lead to sub-optimal performance of domain alignment.
Several latest feature normalization (AutoDIAL, DSBN, and TN) solve the first problems to some extent but do not handle the second issue well.
To handle the two challenges well, we propose RN: through the reciprocity between source and target statistics, RN encourages the statistics of two domains approach each other progressively and leads to better domain alignment eventually. %resulting that the two domain distributions approaching each other.
% With the help of our RN, the source and target features are normalized separately with initial domain statistics at the beginning of training, and then progressively align the domain information via the adaptive reciprocity.
Besides, given different transferability of features from various layers of CNNs, we propose a simple yet effective adaptive gating mechanism to adjust the reciprocity on different layers in an end-to-end way.

%%%%%%%%%%
\begin{figure}
    \centering
    \includegraphics[width=\linewidth]{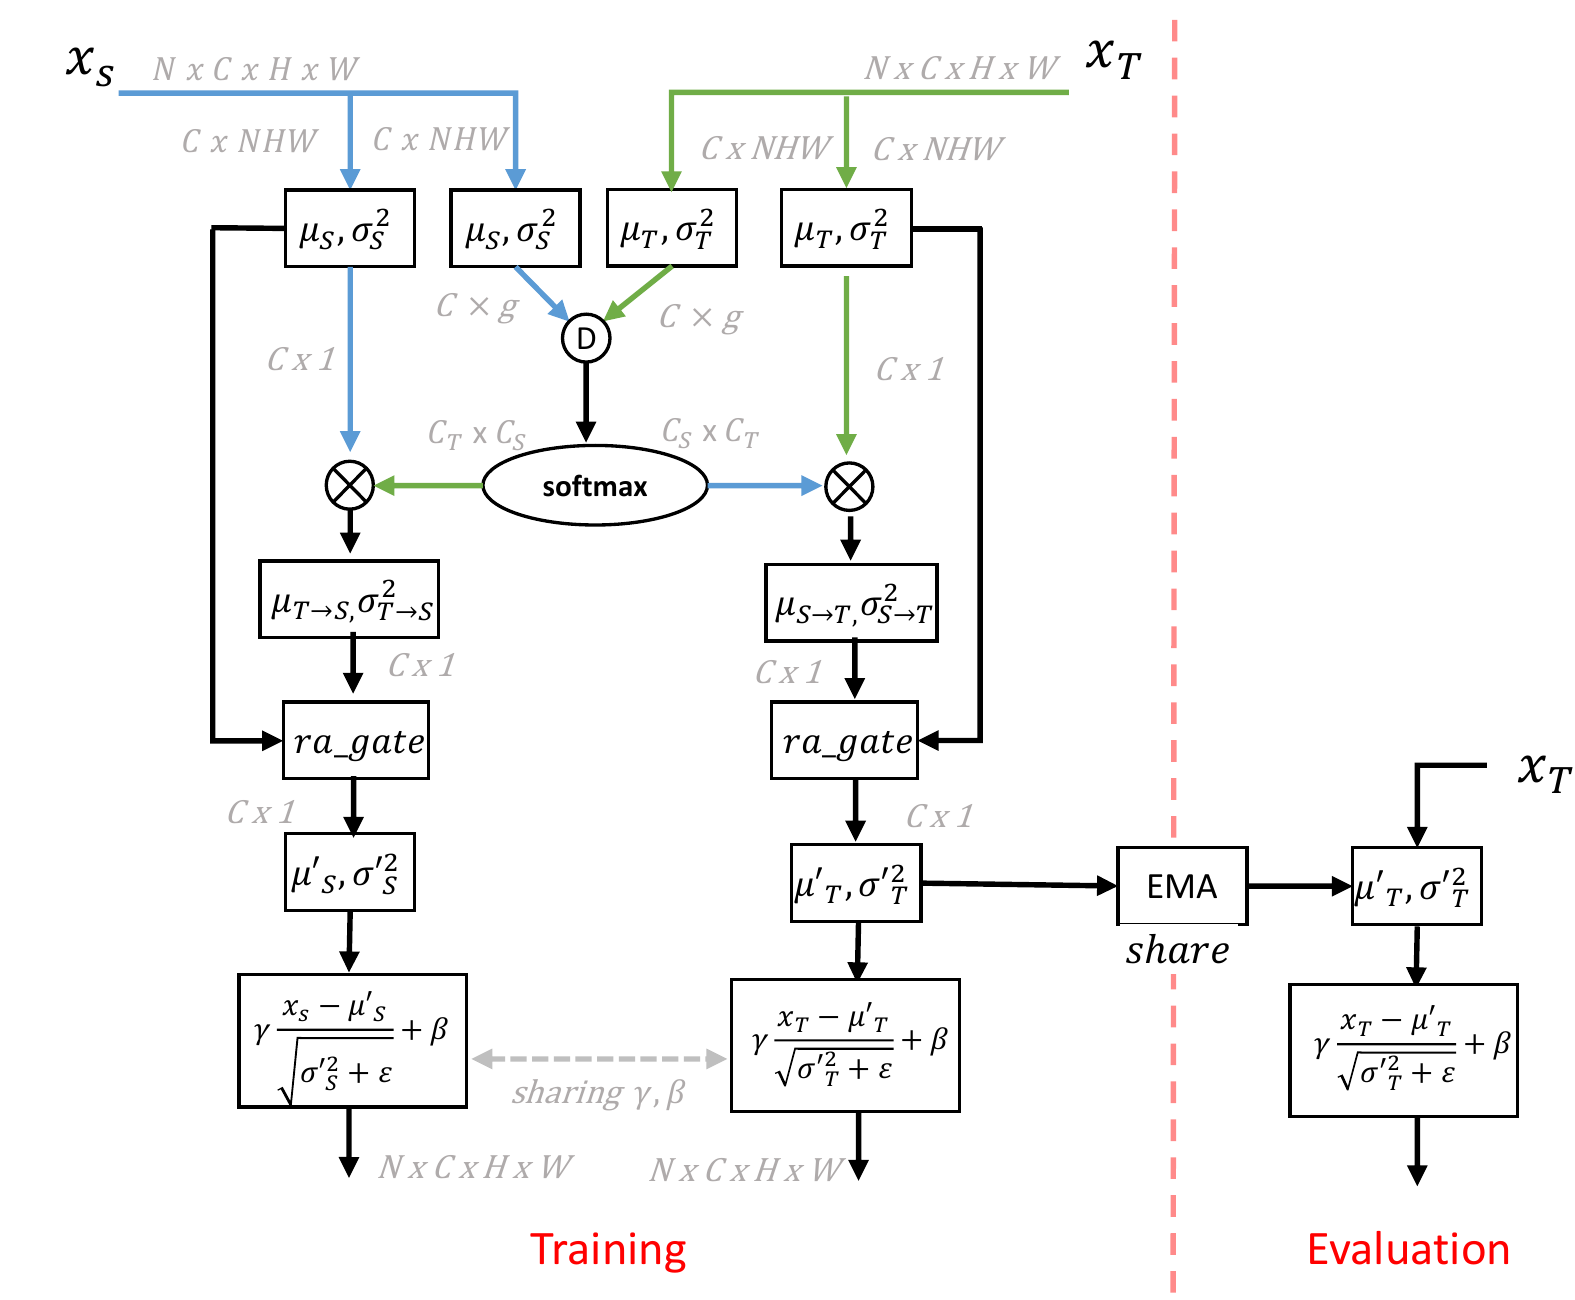}
    \caption{A schematic illustration of the proposed RN. Implementation details in training (\textit{left}) and evaluation (\textit{right}).}
    \label{supfig:process}
    \vspace{-5mm}
\end{figure}

%%%
\subsection{Detailed Formulation}
Figure~\ref{supfig:process} shows a schematic illustration of the proposed RN.

% We supplement complete and brief information for \textbf{Method}.
\myparagraph{Cross-domain Fully-connected Graph (CFG).}
First, we calculate the statistic information of two domains ($\Sdomain$ and $\Tdomain$), $\mu^\Sdomain, (\sigma^2)^\Sdomain$ and $\mu^\Tdomain, (\sigma^2)^\Tdomain$ on each mini-batch:
\begin{equation}
    \mu_{c} = \frac{\sum_{k,i,j}^{B,H,W} x^{\Sdomain}_{kcij}}{BHW}, \  \sigma_{c}^{2} = \frac{\sum_{k,i,j}^{B,H,W} (x^{\Tdomain}_{kcij} - \mu_{c})^{2}}{BHW}.
\label{speq:mu_and_sigma}
\end{equation}

Then we calculate the distance values between statistics of two domains across different channels:
\begin{equation}
    e_{i,j}^{(\mu)} = -(\mu_{i}^{\Sdomain} - \mu_{j}^{\Tdomain})^{2}, \  e_{i,j}^{(\sigma)} = -((\sigma_{i}^{2})^{\Sdomain} - (\sigma_{j}^{2})^{\Tdomain})^{2}.
\end{equation}
In this way, we construct Cross-domain Fully-connected Graph (CFG) with transferability and relevance of each channel.
Next, we obtain the adjacency matrices of Cross-domain Fully-connected Graphs (CFGs):
$E_{\mu}^{\Sdomain \to \Tdomain}$, $E_{\mu}^{\Tdomain \to \Sdomain}$, $E_{\sigma}^{\Sdomain \to \Tdomain}$, and $E_{\sigma}^{\Tdomain \to \Sdomain}$, where $E_{\mu}^{\Sdomain \to \Tdomain} = (E_{\mu}^{\Tdomain \to \Sdomain})^T$ and $E_{\sigma}^{\Sdomain \to \Tdomain} = (E_{\sigma}^{\Tdomain \to \Sdomain})^T$.
The adjacency matrices are used for the reciprocal projection later.
For practical considerations, when the channel dimension is too large ($\eg$ $> 512$), we adopt the group strategy, akin to ~\cite{wu2018GN}.

Then we normalize $E$s row-by-row with softmax for the correlation matrices $\rho_{\mu}^{\Sdomain \to \Tdomain}$, $\rho_{\mu}^{\Tdomain \to \Sdomain}$,  $\rho_{\sigma}^{\Sdomain \to \Tdomain}$ and $\rho_{\sigma}^{\Tdomain \to \Sdomain}$.
Finally, we compute the projections $\tilde{\mu}^{\Sdomain}$, $\tilde{\mu}^{\Tdomain}$, $\tilde{\sigma}^{\Sdomain}$, and $\tilde{\sigma}^{\Tdomain}$:
\begin{equation}
    \tilde{\mu}^{\Sdomain} = \rho_{\mu}^{\Tdomain \to \Sdomain} \otimes \mu^{\Sdomain}, \quad
    \tilde{\mu}^{\Tdomain} = \rho_{\mu}^{\Sdomain \to \Tdomain} \otimes\mu^{\Sdomain},
\end{equation}
\begin{equation}
    (\tilde{\sigma}^{2})^{\Sdomain} = \rho_{\sigma}^{\Tdomain \to \Sdomain} \otimes (\sigma^{2})^{\Sdomain}, \quad
    (\tilde{\sigma}^{2})^{\Tdomain} = \rho_{\sigma}^{\Sdomain \to \Tdomain} \otimes (\sigma^{2})^{\Tdomain},
\end{equation}
where $\otimes$ denotes the matrix multiplication, and $\tilde{x}^{\Sdomain}$ and $\tilde{x}^{\Tdomain}$ denote the projections \textit{from target to source} and the projections \textit{from source to target}, respectively.
In this way, RN conducts the reciprocity by exploiting the transferability and relevance of different channel.

\myparagraph{Reciprocal Aggregation Gate (RA-gate).}
When source and target domains capture the projection information of each other's domain statistics, we propose the RA-gate to aggregate the captured information and the original domain information adaptively.
Specifically, we introduce the learnable gate parameters $g \in [0,1]^C$:
\begin{equation}
    \mu_{agg}^{\Sdomain} = g_{\mu}^{\Sdomain} \cdot \mu^{\Sdomain} + (1-g_{\mu}^{\Sdomain}) \cdot \tilde{\mu}^{\Sdomain},
\end{equation}
\begin{equation}
    \mu_{agg}^{\Tdomain} = g_{\mu}^{\Tdomain} \cdot \mu^{\Tdomain} + (1-g_{\mu}^{\Sdomain}) \cdot \tilde{\mu}^{\Tdomain},
\end{equation}
\begin{equation}
    (\sigma_{agg}^{2})^{\Sdomain} = g_{\sigma}^{\Sdomain} \cdot (\sigma^{2})^{\Sdomain} + (1-g_{\sigma}^{\Sdomain}) \cdot (\tilde{\sigma}^{2})^{\Sdomain},
\end{equation}  
\begin{equation}
    (\sigma_{agg}^{2})^{\Tdomain} = g_{\mu}^{\Tdomain} \cdot (\sigma^{2})^{\Tdomain} + (1-g_{\mu}^{\Sdomain}) \cdot (\tilde{\sigma}^{2})^{\Tdomain}.
\end{equation}

During training RN keeps running estimates of its aggregated mean and variance of each domain via exponential moving average (EMA), similar to BN. Given the $\mu$ and $\sigma$ of the $(t+1)$-th mini-batch of training data, the estimated mean and variance can be calculated by
\begin{equation}
    \hat{\mu}^{\Sdomain}_{new} = (1 - \alpha) \hat{\mu}^{\Sdomain} + \alpha (\mu_{agg}^{\Sdomain})_{t},
\end{equation}
\begin{equation}
    \hat{\mu}^{\Tdomain}_{new} = (1 - \alpha) \hat{\mu}^{\Tdomain} + \alpha (\mu_{agg}^{\Tdomain})_{t},
\end{equation}
\begin{equation}
    (\hat{\sigma}^{2})^{\Sdomain}_{new} = (1 - \alpha) (\hat{\sigma}^{2})^{\Sdomain} + \alpha (\sigma_{agg}^{2})^{\Sdomain})_{t},
\end{equation}
\begin{equation}
    (\hat{\sigma}^{2})^{\Tdomain}_{new} = (1 - \alpha) ((\hat{\sigma}^{2})^{\Tdomain} + \alpha ((\sigma_{agg}^{2})^{\Tdomain})_{t},
\end{equation}
where $\alpha$ is a hyper-parameter and initialized to $0.1$, and $(\cdot)_{t}$ denotes the statistic information after $t$ training iterations.
This strategy enables RN to utilize the estimated domain statistics directly to normalize the examples without performing extra calculations during the evaluation phase.

%%%%%%%
\input{latex/tabs/Supplement_TestTime}

\myparagraph{Separate Normalization.}
To address the first limitation of BN, we adopt the aggregated domain statistics to normalize the features from two domains, separately:
\begin{equation}
    \tilde{x}_{nc}^{\Sdomain} = \gamma_{c} \bar{x}_{nc}^{\Sdomain} + \beta_{c}, \quad
    \tilde{x}_{nc}^{\Tdomain} = \gamma_{c} \bar{x}_{nc}^{\Tdomain} + \beta_{c},
\end{equation}
\begin{equation}
    \bar{x}_{nc}^{\Sdomain}=\frac{x_{nc}^{\Sdomain}-\mu_{agg,nc}^{\Sdomain}}{\sqrt{(\sigma_{agg, nc}^{2})^{\Sdomain} + \epsilon}}, 
    \
    \bar{x}_{nc}^{\Tdomain}=\frac{x_{nc}^{\Tdomain}-\mu_{agg,nc}^{\Tdomain}}{\sqrt{(\sigma_{agg, nc}^{2})^{\Tdomain} + \epsilon}},
\end{equation}
where $\epsilon$ is a small constant to avoid divide-by-zero.

Overall, as shown in Figure~\ref{supfig:process}, RN calculates the statistics of two domains separately and conducts reciprocity according to the \textit{transferability} and \textit{relevance} of various channel. After CFGs, the original and projection statistics are adaptively aggregated via RA-gate. Finally, the new statistics of two domains are used to normalize source and target features separately for the sake of domain-specific knowledge.

%%%
% \subsection{Flow Diagram }
% \input{latex/secs/3__algorithm}

%%%
\subsection{Computational Complexity}
\paragraph{Theoretical} Our RN has a relatively low computational complexity. For the RN at layer $l$, the amount of introduced parameters is $N_{l}=4C_{l}$, where $C_l$ denotes the number of channels at layer $l$.
In each RN, the computation involves two linear multiplication. %That is, our RN introduces reasonable number of parameters and obtains promising improvement.
During the evaluation, the computational complexity of RN is exactly the same as BN.

\myparagraph{Quantitative}
We compare the classification performance and test time of different methods in Table~\ref{spptab:test_time}. Generally, our RN costs the least test time which is the same as that of BN, whil TN is more \textit{ten times} slower than BN. %although TN does not introduce extra parameters. This maybe because the real-time computation in TN is relative large during evaluation phase.
DSBN also conduct one typical BN operation at evaluation but it needs extra time to judge whether the features come from source or target domains. 
% Particularly, as the amount of data smaller, RN even achieves less test time than BN. 
Therefore, our RN achieves both better performance and less test time, which is significant for industrial applications.
%In practice, we find it is not necessary for the neurons to communicate at all layers. The complexity is further limited by adding our NC block to only a few separate layers.

%%%
\subsection{Descriptions of Code}
In the \textit{CodeAndDataAppendix} of our supplementary material, we upload a complete project in one zip file. \textit{reciprocal\_norm.py} contains detailed implementations of the proposed RN. We also have several \textit{run\_X-Y.sh} shell that shows how to reproduce the performance of the corresponding tasks, $\ie$ X $\to$ Y and Y $\to$ X, from Office-Home dataset.
