# Supplementary material for: Reciprocal Normalization for Domain Adaptation
Source: arXiv:2112.10474 source file (2021-12-20)
Supplement: Supplementary file 2 [file Details_Officehome.tex]

%% without reference
\begin{table*}
    \centering
    % \setlength{\abovecaptionskip}{0pt}
    % \captionsetup{font={footnotesize}}
    \footnotesize{
    \setlength{\tabcolsep}{0.9mm}{
    \caption{UDA accuracy ($\%$) of different feature normalization methods on Office-Home (ResNet-50).}
    \label{subtab:OfficeHome_results}
    \begin{tabular}{lccccccccccccc}
        \toprule
        Method & Ar$\to$Cl & Ar$\to$Pr & Ar$\to$Rw & Cl$\to$Ar & Cl$\to$Pr & Cl$\to$Rw & Pr$\to$Ar & Pr$\to$Cl & Pr$\to$Rw & Rw$\to$Ar & Rw$\to$Cl & Rw$\to$Pr & AVG \\
        % \midrule
        % \multicolumn{14}{c}{ResNet-50} \\
        \midrule
        ResNet-50 (source only) & 34.9 & 50.0 & 58.0 & 37.4 & 41.9 & 46.2 & 38.5 & 31.2 & 60.4 & 53.9 & 41.2 & 59.9 & 46.1 \\
        \midrule
        DANN(+BN) & 45.9 & 61.2 & 68.9 & 50.4 & 59.7 & 61.0 & 45.8 & 43.4 & 70.3 & 63.9 & 52.4 & 76.8 & 58.3 \\
        DANN+AutoDIAL & 51.1 & 61.4 & 71.6 & 48.0 & 58.0 & 60.2 & 48.5 & 44.3 & 70.9 & 63.1 & 50.7 & 78.0 & 58.8 \\
        DANN+DSBN & 42.9 & 59.7 & 68.4 & 47.5 & 58.9 & 59.3 & 44.5 & 36.6 & 69.6 & 56.7 & 44.4 & 69.5 & 54.8 \\
        DANN+TN & 43.5 & 60.9 & 72.1 & 51.0 & 61.5 & 62.5 & 49.6 & 46.8 & 70.4 & 63.7 & 52.2 & 77.9 & 59.3 \\
        DANN+RN & \textbf{47.3} & \textbf{63.1} & \textbf{74.4} & \textbf{57.1} & \textbf{64.7} & \textbf{68.4} & \textbf{55.2} & \textbf{47.8} & \textbf{75.9} & \textbf{68.9} & \textbf{53.5} & \textbf{79.3} & \textbf{63.0} \\
        \midrule
        CDAN(+BN) & 50.7 & 70.6 & 76.0 & 57.6 & 70.0 & 70.0 & 57.4 & 50.9 & 77.3 & 70.9 & 56.7 & 81.6 & 65.8 \\
        CDAN+AutoDIAL & 49.8 & 69.8 & 76.2 & 59.6 & 70.4 & 69.2 & 57.6 & 51.8 & 76.0 & 71.2 & 57.5 & 81.4 & 65.9 \\
        CDAN+DSBN & 47.5 & 72.6 & 76.5 & 57.0 & 68.3 & 70.0 & 58.3 & 37.7 & 78.4 & 70.2 & 51.4 & 78.4 & 64.7 \\
        CDAN+TN & 50.2 & 71.4 & 77.4 & 59.3 & 72.7 & 73.1 & 61.0 & 53.1 & 79.5 & 71.9 & 59.0 & 82.9 & 67.6 \\
        CDAN+RN & \textbf{55.6} & \textbf{72.6} & \textbf{78.1} & \textbf{65.7} & \textbf{74.7} & \textbf{74.5} & \textbf{66.2} & \textbf{57.1} & \textbf{82.0} & \textbf{75.2} & \textbf{60.5} & \textbf{84.6} & \textbf{70.6} \\
        % @ 200729, PDA later
        \bottomrule
    \end{tabular}
    } % setlength
    } % footnotesize
    \vspace{-3mm}
\end{table*}
