# Supplementary material for: Reciprocal Normalization for Domain Adaptation
Source: arXiv:2112.10474 source file (2021-12-20)
Supplement: Supplementary file 3 [file Details_Visda.tex]

%% without reference
\begin{table*}
    \centering
    % \setlength{\abovecaptionskip}{0pt}
    % \captionsetup{font={footnotesize}}
    \footnotesize{
    \caption{The Detailed class-wise accuracy (\%) on VisDA-C.}
    \label{subtab:ResultsOnVisDA2017}
    \begin{tabular}{lccccccccccccc}
        \toprule
        % \textbf{ResNet-101} & \rotatebox{90}{aeroplane} & \rotatebox{90}{bicycle} & \rotatebox{90}{bus} & \rotatebox{90}{car} & \rotatebox{90}{horse} & \rotatebox{90}{knife} & \rotatebox{90}{motorcycle} & \rotatebox{90}{person} & \rotatebox{90}{plant} & \rotatebox{90}{skateboard} & \rotatebox{90}{train} & \rotatebox{90}{truck} & AVG \\
        \textbf{ResNet-101} & aero. & bike & bus & car & horse & knife & motor. & person & plant & sktb. & train & truck & AVG \\
        \midrule
        source only & 55.1 & 53.3 & 61.9 & 59.1 & 80.6 & 17.9 & 79.7 & 31.2 & 81.0 & 26.5 & 73.5 & 8.5 & 52.4 \\
        \midrule
        DANN(+BN) & 81.9 & 77.7 & \textbf{82.8} & 44.3 & 81.2 & 29.5 & 65.1 & 28.6 & 51.9 & \textbf{54.6} & \textbf{82.8} & 7.8 & 57.4 \\
        DANN+AutoDIAL & 86.5 & \textbf{94.4} & 61.8 & 74.3 & 95.5 & 25.9 & 59.9 & 62.3 & 80.0 & 28.7 & 71.6 & 35.9 & 64.7 \\
        DANN+DSBN & 84.0 & 83.9 & 72.0 & 75.8 & 95.2 & \textbf{61.6} & 44.8 & 60.8 & 91.4 & 41.2 & 76.3 & 48.5 & 69.6 \\
        % +TN &  &  &  &  &  &  &  &  &  &  &  &  &  \\
        DANN+RN & \textbf{90.4} & 92.7 & 71.9 & \textbf{84.5} & \textbf{96.6} & 30.2 & \textbf{81.4} & \textbf{67.9} & \textbf{95.0} & 49.2 & 73.9 & \textbf{64.8} & \textbf{74.9} \\
        \midrule
        CDAN(+BN) & 85.2 & 66.9 & \textbf{83.0} & 50.8 & 84.2 & \textbf{74.9} & \textbf{88.1} & 74.5 & 83.4 & 76.0 & 81.9 & 38.0 & 73.9 \\
        DANN+AutoDIAL & 92.8 & 94.8 & 66.5 & 74.3 & 92.4 & 51.8 & 68.3 & 60.7 & 88.4 & 54.9 & \textbf{85.4} & 61.2 & 74.5 \\
        DANN+DSBN & 88.2 & 91.0 & 79.3 & \textbf{85.5} & 93.7 & 70.7 & 57.2 & \textbf{74.2} & 91.7 & 78.0 & 81.4 & 52.3 & 78.6 \\
        % +TN &  &  &  &  &  &  &  &  &  &  &  &  &  \\
        DANN+RN & 96.7 & 94.3 & 70.4 & 84.4 & \textbf{96.6} & 36.4 & 81.8 & 68.9 & 95.4 & 81.5 & 77.9 & 77.0 & \textbf{80.1} \\
        % CDAN+RN$^\star$ & \textbf{97.8} & \textbf{97.6} & 63.4 & 74.2 & 96.4 & 23.5 & 70.4 & 72.7 & \textbf{97.4} & \textbf{89.6} & 83.0 & \textbf{94.0} & 80.0 \\
        % \midrule
        % \textbf{ResNet-50} & aeroplane & bicycle & bus & car & horse & knife & motorcycle & person & plant & skateboard & train & truck & AVG \\
        % \midrule
        % source-only &  &  &  &  &  &  &  &  &  &  &  &  &  \\
        % \midrule
        % CDAN(+BN) &  &  &  &  &  &  &  &  &  &  &  &  &  \\
        % CDAN+AutoDIAL &  &  &  &  &  &  &  &  &  &  &  &  &  \\
        % CDAN+DSBN &  &  &  &  &  &  &  &  &  &  &  &  &  \\
        % CDAN+TN &  &  &  &  &  &  &  &  &  &  &  &  &  \\
        % CDAN+RN & 96.6 & 92.5& 77.5 & 81.2 & 94.6 & 26.6 & 84.2 & 64.1 & 94.6 & 83.8 & 81.0 & 84.9 &  79.6\\
        % CDAN+RN$^\star$ & 95.6 & 97.7 & 56.9 & 75.6 & 96.4 & 21.8 & 75.8 & 67.5 & 95.2 & 76.2 & 82.2  & 90.3 & 75.6 \\
        \bottomrule
    \end{tabular}
    % } % setlength
    } % footnotesize
    \vspace{-2mm}
\end{table*}
