# Supplementary material for: Reciprocal Normalization for Domain Adaptation
Source: arXiv:2112.10474 source file (2021-12-20)
Supplement: Supplementary file 5 [file Gate_visualization.tex]

\input{latex/figs/Supplyment_Gate}
