# Supplementary material for: Reciprocal Normalization for Domain Adaptation
Source: arXiv:2112.10474 source file (2021-12-20)
Supplement: Supplementary file 6 [file Supplement_difflayers.tex]

\begin{figure*}
  \centering
    \begin{minipage}{0.82\linewidth}
        \includegraphics[width=1\linewidth]{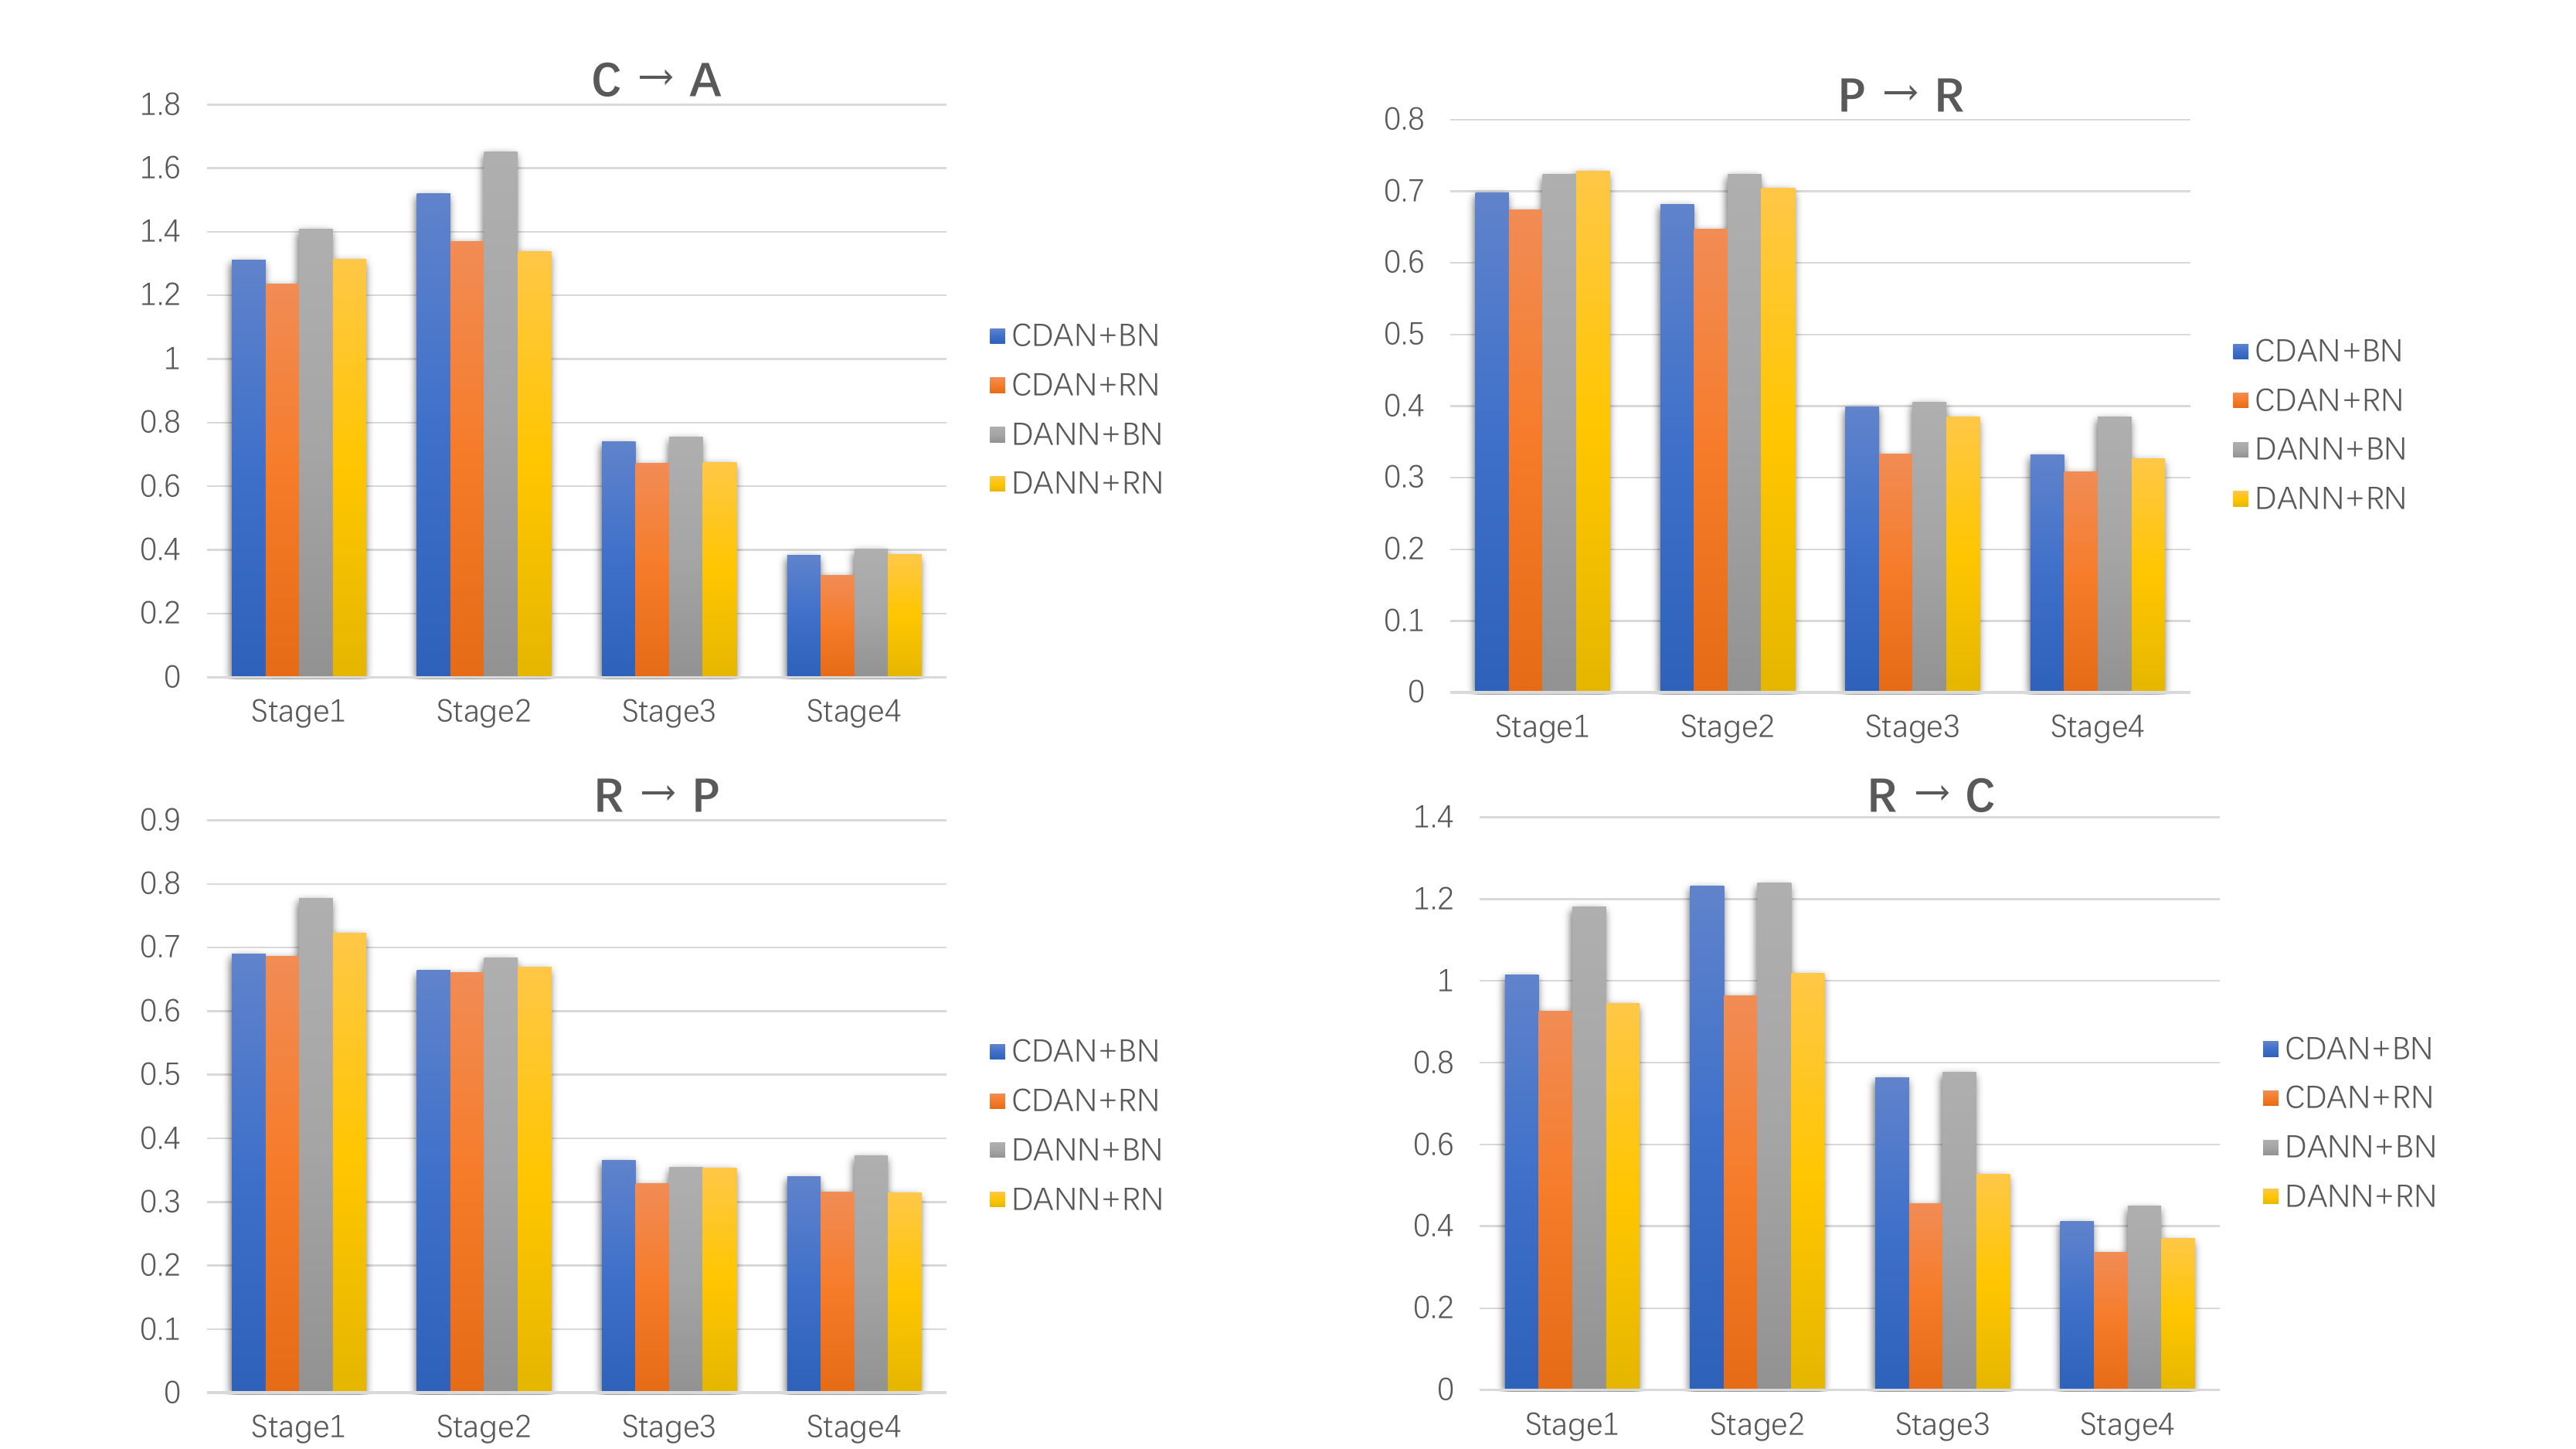}
    \end{minipage}
    \begin{minipage}{0.82\linewidth}
        \includegraphics[width=1\linewidth]{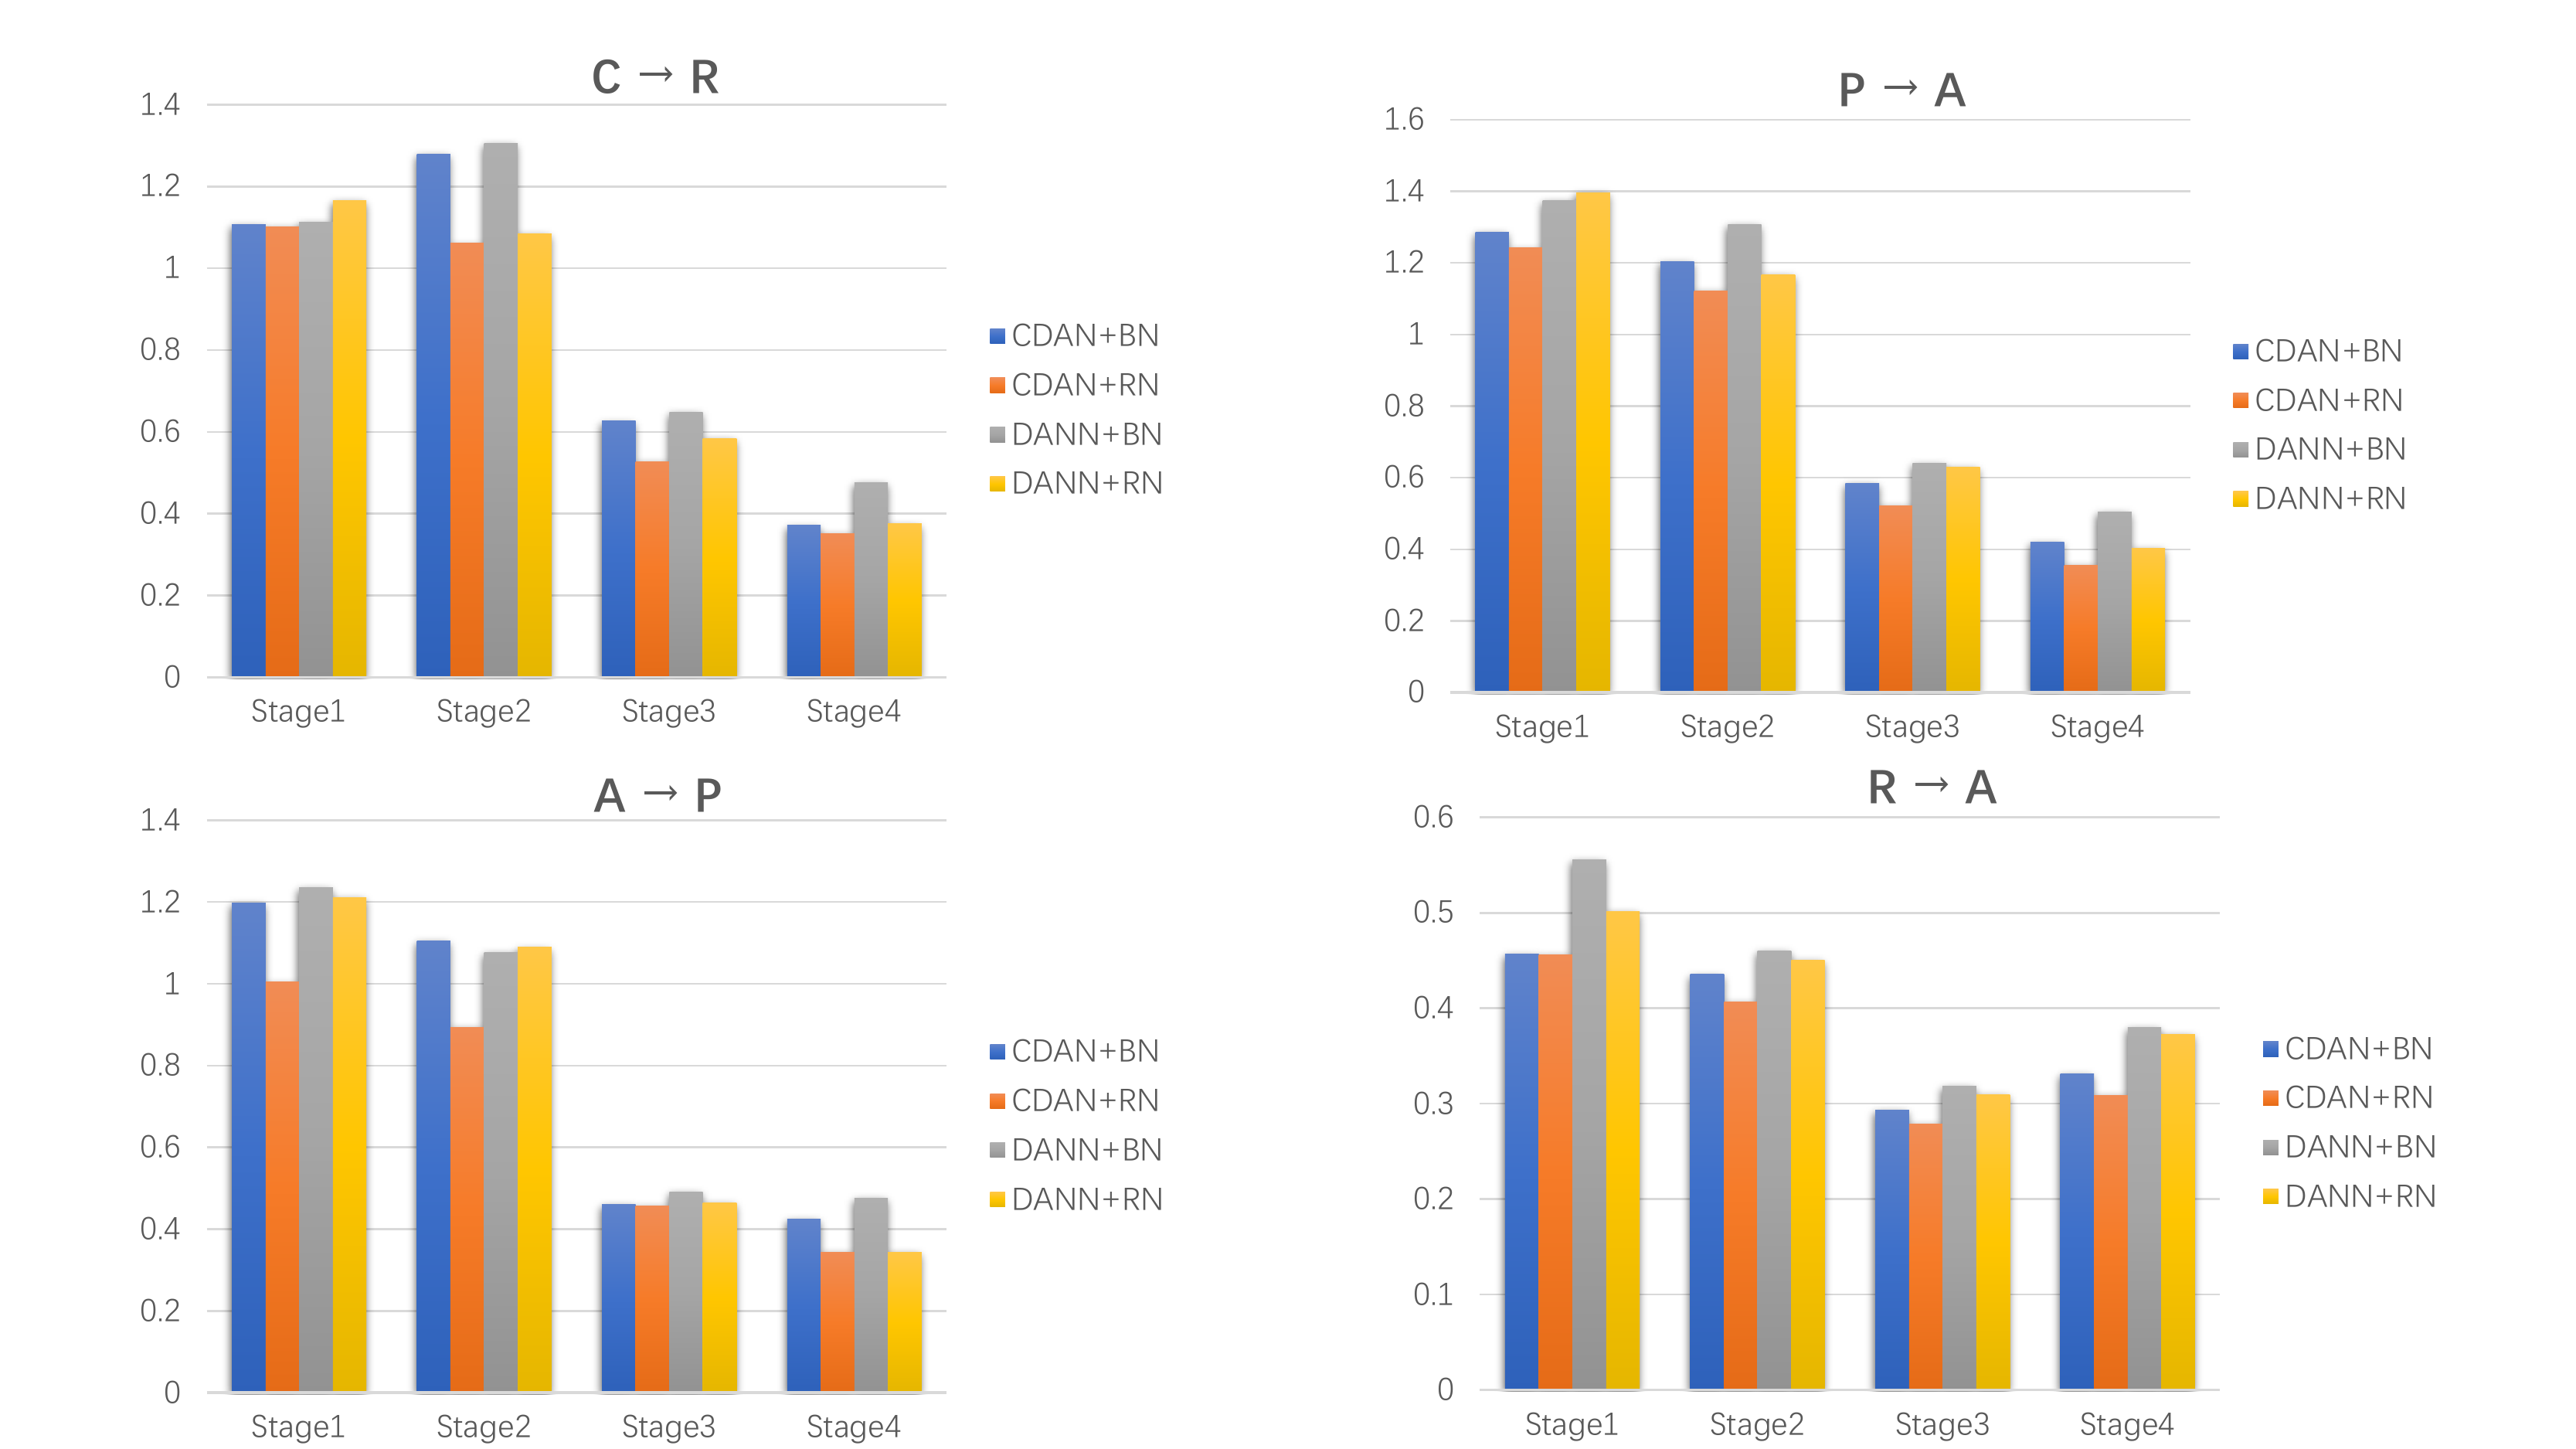}
    \end{minipage}
     \begin{minipage}{\linewidth}
        \includegraphics[width=1\linewidth]{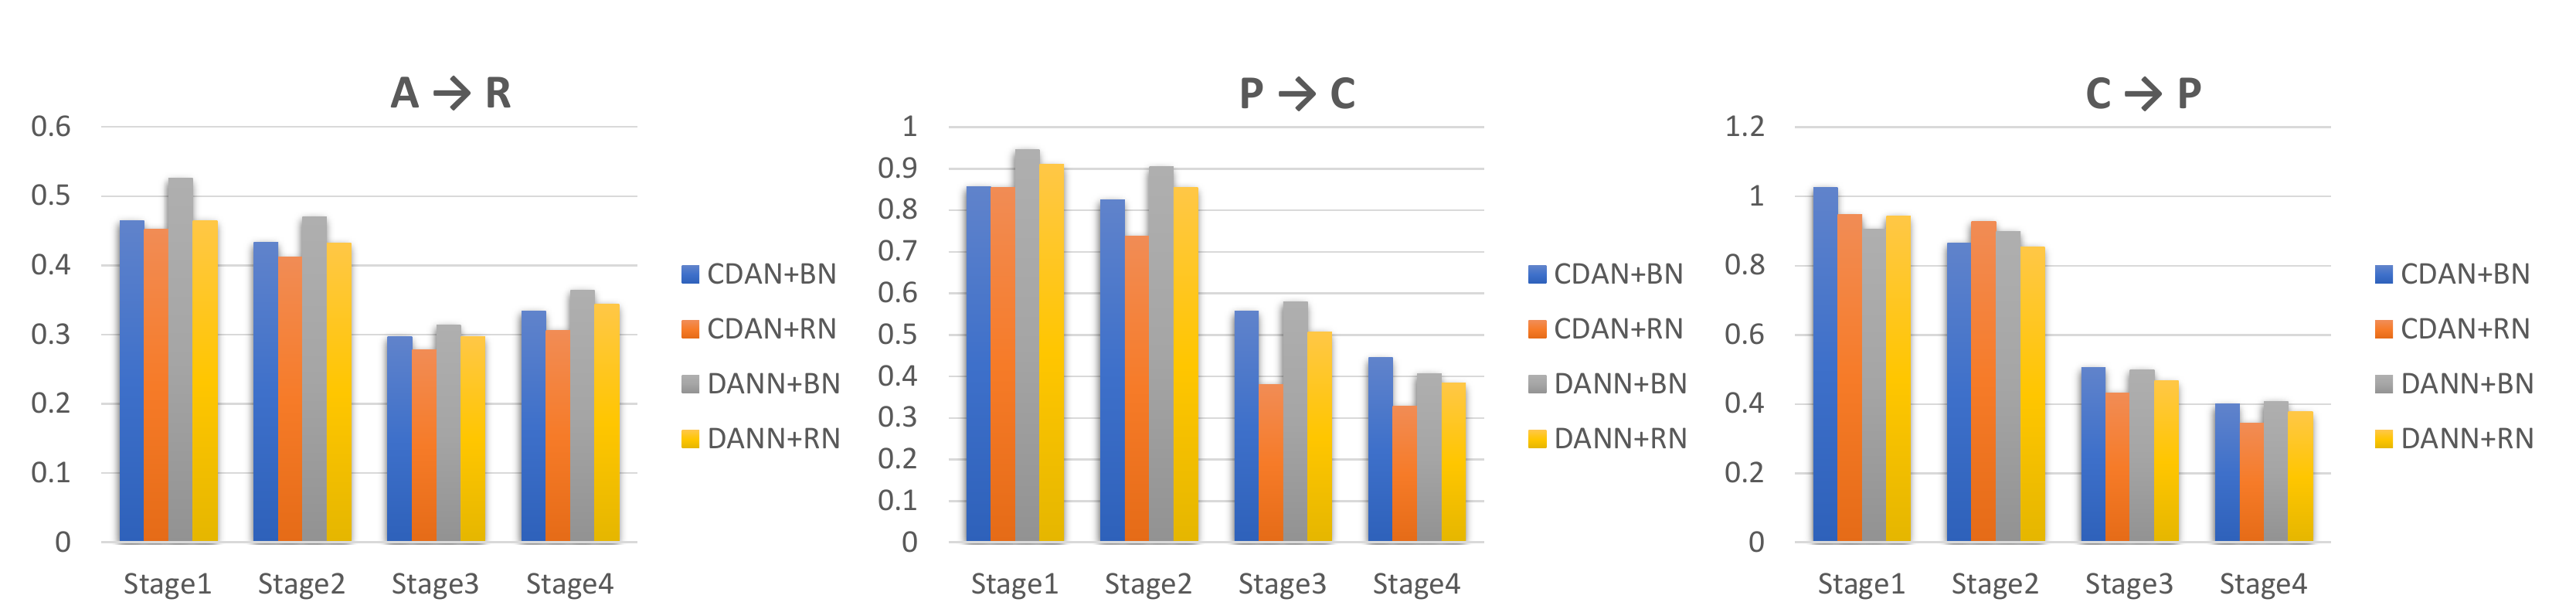}
    \end{minipage}
  \caption{Visualization results of domain discrepancy (MMD scores) of intermediate layers, $\ie$ the four stages in ResNet-50, on the other $11$ transfer tasks (except A $\to$ C) on Office-Home.}
	\label{subfig:difflayers}
% 	\vspace{0.2in}
\end{figure*}
