# Supplementary material for: Reciprocal Normalization for Domain Adaptation
Source: arXiv:2112.10474 source file (2021-12-20)
Supplement: Supplementary file 7 [file Supplement_process.tex]

\begin{figure}
    \centering
    \includegraphics[width=\linewidth]{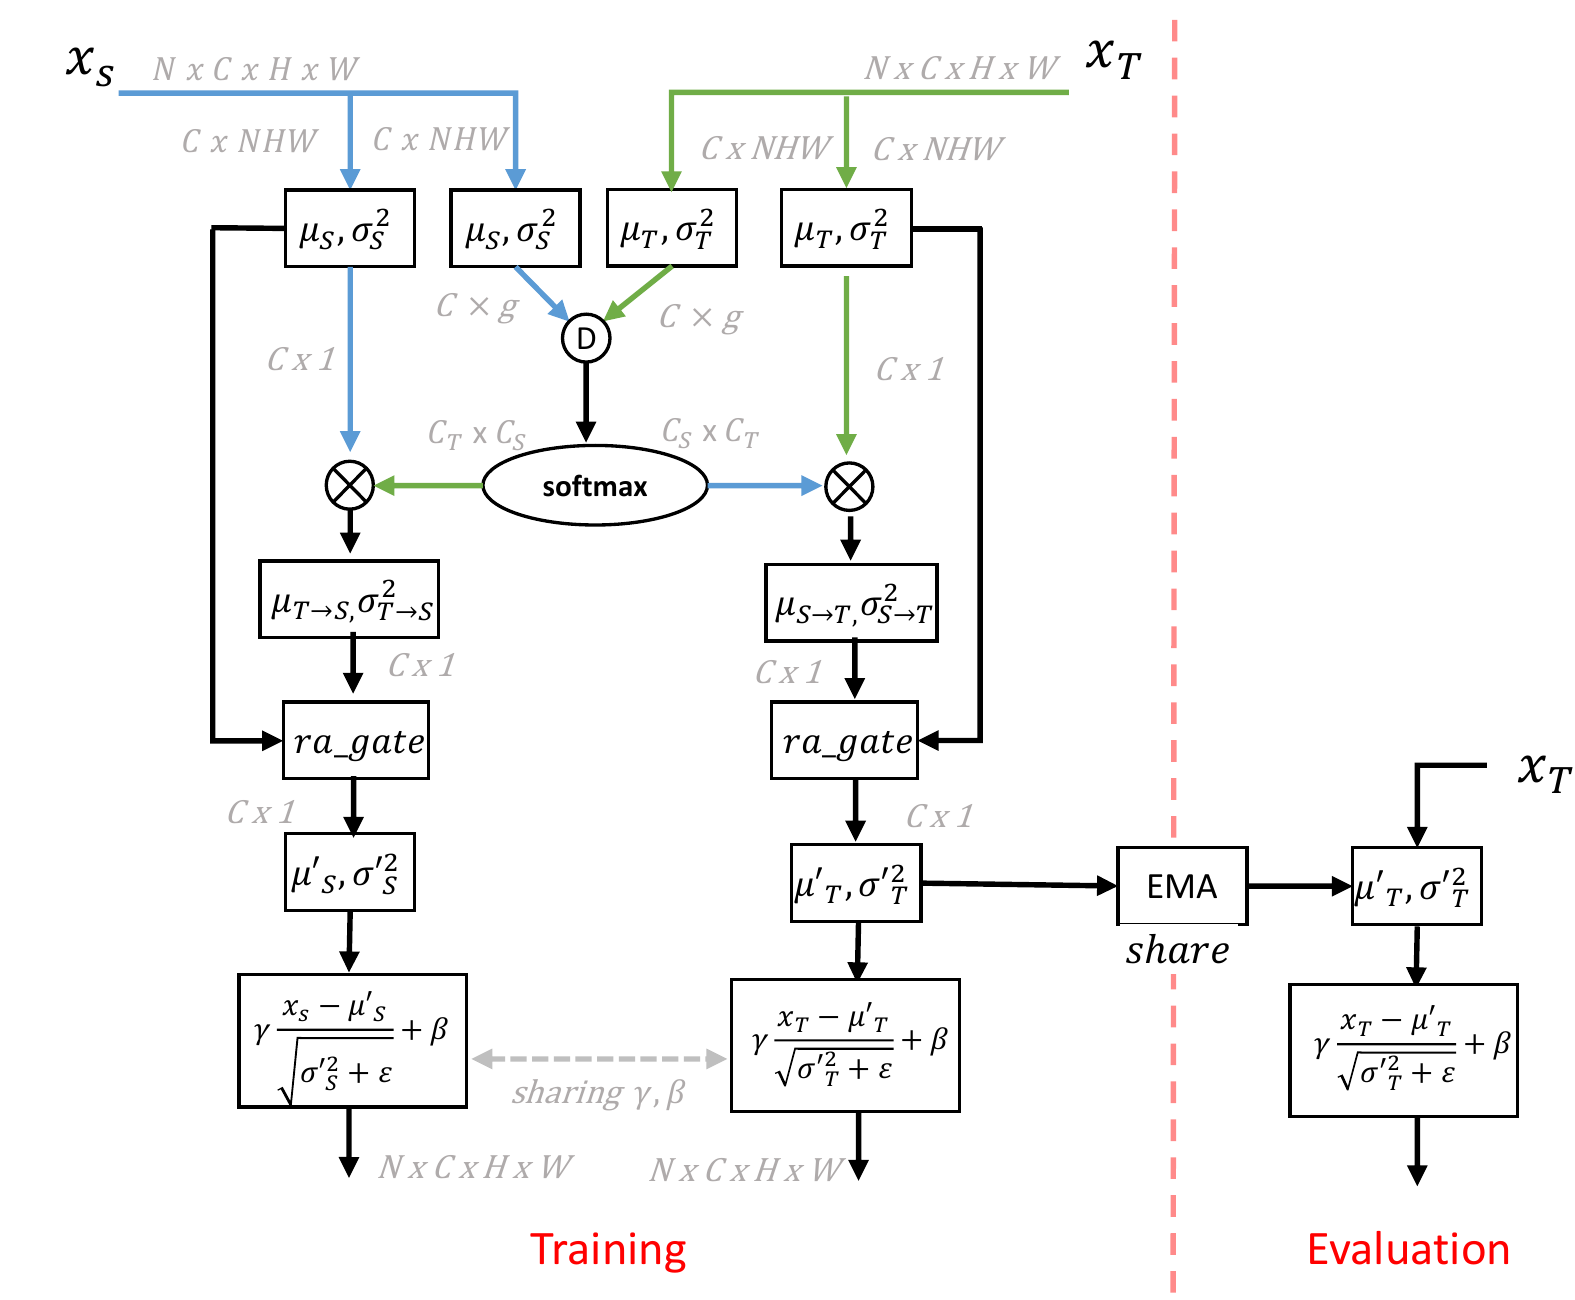}
    \caption{A schematic illustration of the proposed RN. Implementation details in training (\textit{left}) and evaluation (\textit{right}).}
    \label{supfig:process}
    \vspace{-5mm}
\end{figure}
