# Supplementary material for: Reciprocal Normalization for Domain Adaptation
Source: arXiv:2112.10474 source file (2021-12-20)
Supplement: Supplementary file 11 [file Supplement_layers_ablation.tex]

\begin{table}
    \centering
    \caption{Ablation study of RN on different intermediate layers. Experiments are conducted with CDAN (UDA) on $3$ randomly selected transfer tasks from Office-Home (ResNet-50). 
    %The random seed is \textit{2021}.
    }
    \label{subtab:AblationOnEachLayer}
    \footnotesize{
    \setlength{\tabcolsep}{1.8mm}{
    \begin{tabular}{cccc||ccc}
        \toprule
        \multicolumn{4}{c||}{layer configuration} & \multicolumn{3}{c}{transfer task} \\
        Layer 1 & Layer 2 & Layer 3 & Layer 4 & A$\to$C & C$\to$P & A$\to$R \\
        \hline
       \checkmark  &  &  &                       & 50.7 & 72.7 &  77.6 \\
         & \checkmark  &  &                       & 51.2 & 72.2 &  77.3 \\
         &  & \checkmark  &                       & 52.3 & 72.7 &  77.4 \\
         &  &  & \checkmark                       & 52.5 & 72.1 &  77.7 \\
         &  & \checkmark  & \checkmark               & 56.0 & 72.3 &  77.7 \\
         & \checkmark  & \checkmark  & \checkmark         & 56.1 & 73.6 &  77.9 \\
        \checkmark  & \checkmark  & \checkmark  & \checkmark  & 56.2 & 74.7 &  78.1 \\
        \bottomrule
    \end{tabular}
    }
    }
\end{table}
