# Supplementary material for: Reciprocal Normalization for Domain Adaptation
Source: arXiv:2112.10474 source file (2021-12-20)
Supplement: Supplementary file 12 [file Diff_Layers.tex]

\input{latex/figs/Supplement_difflayers}
